# Supplementary material for: Studying continuous, time-varying, and/or complex exposures using longitudinal modified treatment policies
Source: arXiv:2304.09460 source file (2024-05-14)
Supplement: Supplementary file 4 [file appendix.tex]

\documentclass[12pt]{article}
\usepackage{mathtools}
\usepackage{graphicx}
\usepackage[super,comma,sort&compress]{natbib}
\usepackage[margin=1in]{geometry}
\usepackage[english]{babel}
\usepackage{longtable}
\usepackage{color}
\usepackage{float}
\usepackage{amssymb,amsmath,amsthm}
\usepackage{multirow}
\usepackage[titletoc,title]{appendix}
\usepackage{authblk}
\usepackage{setspace}
\usepackage{dsfont}
\usepackage[OT1]{fontenc}
\usepackage{refcount}
\usepackage[colorlinks,citecolor=blue,urlcolor=blue]{hyperref}
\usepackage{float}
\usepackage{mathrsfs}
\usepackage{tabulary}
\usepackage{rotating}
\usepackage{setspace}
\usepackage{multirow}
\usepackage{paralist}
\usepackage{booktabs}
\usepackage{bm}
\usepackage{longtable}
\usepackage{bbm}
\usepackage{setspace}
\usepackage{array}
\usepackage{makecell}

\usepackage{utfsym}
\usepackage{makecell}
\usepackage{adjustbox}
\usepackage{listings}
\usepackage{lscape}
\usepackage[T1]{fontenc}
\usepackage[utf8]{inputenc}
\usepackage[english]{babel}
\setlength{\parindent}{4em}
\usepackage{dsfont}
\usepackage{hyperref}
\usepackage[para]{threeparttable} % kat added 
\usepackage{quiver}

\usepackage{url}
\usepackage{booktabs}
\usepackage{authblk}
\usepackage{etoolbox}
\usepackage{longtable}
\usepackage{caption}
\usepackage{hyperref}
\usepackage{nameref,zref-xr} % nameref before zref-xr
\zxrsetup{toltxlabel} % allows to use the \ref command as usual
